# Supplementary material for: Bootstrapping Chest CT Image Understanding by Distilling Knowledge from X-ray Expert Models
Source: arXiv:2404.04936 source file (2024-04-07)
Supplement: Supplementary file 1 [file X_suppl_old.tex]

\clearpage
\setcounter{page}{1}
\maketitlesupplementary



\section{Related key words and distribution of six pathologies}
We utilized the CheXpert labeling tool~\cite{irvin2019chexpert} to extract six pathologies from the reports. For each CT report, we employed specific keywords to target six distinct pathologies, as outlined in Table~\ref{tab.key_words}. The distribution and number of these six pathologies within ChesstCT-16K and ChestCT-EXT datasets are presented in Table~\ref{tab.pathology_number}.


\begin{table}[H]
\small
\centering
\begin{tabular}{l|clllll}
\hline
Pythology        & \multicolumn{6}{c}{Related key words}                                                                                                                                                                                                                                                                                                                                                                                             \\ \hline
Nodule           & \multicolumn{6}{c}{nodule, nodules, nodular}                                                                                                                                                                                                                                                                                                                                                                                      \\ \hline
Opacity          & \multicolumn{6}{c}{\begin{tabular}[c]{@{}c@{}}opacity, opacities, decreased  translucency, \\ increased density,  airspace disease, \\ air-space disease, air space \\ disease, infiltrate, infiltration, \\ interstitial marking,  interstitial pattern, \\ interstitial lung, reticular pattern, \\ reticular marking, reticulation, \\ parenchymal scarring,  peribronchial \\ thickening, wall thickening, scar\end{tabular}} \\ \hline
Pleural Effusion & \multicolumn{6}{c}{pleural   fluid, pleural effusion}                                                                                                                                                                                                                                                                                                                                                                             \\ \hline
Emphysema        & \multicolumn{6}{c}{emphysema}                                                                                                                                                                                                                                                                                                                                                                                                     \\ \hline
Inflammation     & \multicolumn{6}{c}{\begin{tabular}[c]{@{}c@{}}inflammation, pneumonia, \\      infection, infectious \\      process, infectious\end{tabular}}                                                                                                                                                                                                                                                                                    \\ \hline
Calcification    & \multicolumn{6}{c}{calcification,   calcifications}                                                                                                                                                                                                                                                                                                                                                                               \\ \hline
\end{tabular}
\caption{Related key words for six pathologies used in CheXpert labeling tool.}
\label{tab.key_words}
\end{table}


\begin{table}[H]
\small
\centering
\begin{tabular}{l|ccc|c}
\toprule
\multirow{2}{*}{Pythology} & \multicolumn{3}{c|}{ChestCT-16K} & ChestCT-EXT \\
                           & Train      & Val      & Test     & Test        \\ \midrule
Nodule                     & 8084       & 923      & 1894     & 1689        \\
Opacity                    & 6559       & 757      & 1489     & 1347        \\
Pleural Effusion           & 536        & 65       & 120      & 147         \\
Emphysema                  & 522        & 57       & 95       & 221         \\
Inflammation               & 1244       & 139      & 303      & 220         \\
Calcification              & 1826       & 182      & 384      & 290         \\ \bottomrule
\end{tabular}
\caption{Pathology numbers in ChestCT-16K dataset and ChestCT-EXT dataset.}
\label{tab.pathology_number}
\end{table}






\section{NLP metrics of report generation task}
In the context of the report generation task, we have included NLP metrics to evaluate the proposed method. Table~\ref{tab.nlp_results} showcases the outstanding performance of our method, consistently outperforming other methods across all NLP metrics, not only on the internal test set, ChestCT-16K, but also on the external test set, ChestCT-EXT. These experimental results provide compelling evidence for the superiority and robustness of our method.


\begin{table}[]
\small
\centering
\begin{tabular}{lcccc}
\toprule
\multicolumn{1}{l|}{Methods} & BLEU-4 & METEOR & ROUGE-L & CIDEr \\ \hline
\multicolumn{5}{c}{Internal test: ChestCT-16K}                   \\ \toprule
\multicolumn{1}{l|}{R2Gen~\cite{R2Gen}}   & 7.3    & 10.4   & 28.3    & 7.8   \\
\multicolumn{1}{l|}{CMN~\cite{R2Gen-CMN}}     & 5.6    & 8.6    & 25.5    & 5.2   \\
\multicolumn{1}{l|}{RadFM~\cite{RadFM}}   & 0.1    & 4.3    & 8.6     & 1.5   \\
\multicolumn{1}{l|}{BLIP~\cite{BLIP}}    & 13.2   & 19.4   & 37.9    & 21.1  \\
\multicolumn{1}{l|}{DCL~\cite{DCL}}     & 12.5   & 18.6   & 37.1    & 19.0  \\ \midrule
\multicolumn{1}{l|}{Ours}    & \textbf{13.8}   & \textbf{21.3}   & \textbf{40.2}    & \textbf{24.4}  \\ \bottomrule
\multicolumn{5}{c}{External test: ChestCT-EXT}                   \\ \toprule
\multicolumn{1}{l|}{R2Gen~\cite{R2Gen}}   & 6.9    & 10.8   & 27.1    & 3.7   \\
\multicolumn{1}{l|}{CMN~\cite{R2Gen-CMN}}     & 3.2    & 7.2    & 21.3    & 1.7   \\
\multicolumn{1}{l|}{RadFM~\cite{RadFM}}   & 0.1    & 0.7    & 1.6     & 0.2   \\
\multicolumn{1}{l|}{BLIP~\cite{BLIP}}    & 11.2   & 16.7   & 33.8    & 9.6   \\
\multicolumn{1}{l|}{DCL~\cite{DCL}}     & 10.6   & 16.4   & 33.6    & 9.9   \\ \midrule
\multicolumn{1}{l|}{Ours}    & \textbf{12.0}   & \textbf{17.6}   & \textbf{35.4}    & \textbf{10.7}  \\ \bottomrule
\end{tabular}
\caption{Natural language generation metrics of the report generation task on the ChestCT-16K test set and ChestCT-EXT dataset.}
\label{tab.nlp_results}
\end{table}





\begin{figure*}
    \centering
    \includegraphics[width=1.0\linewidth]{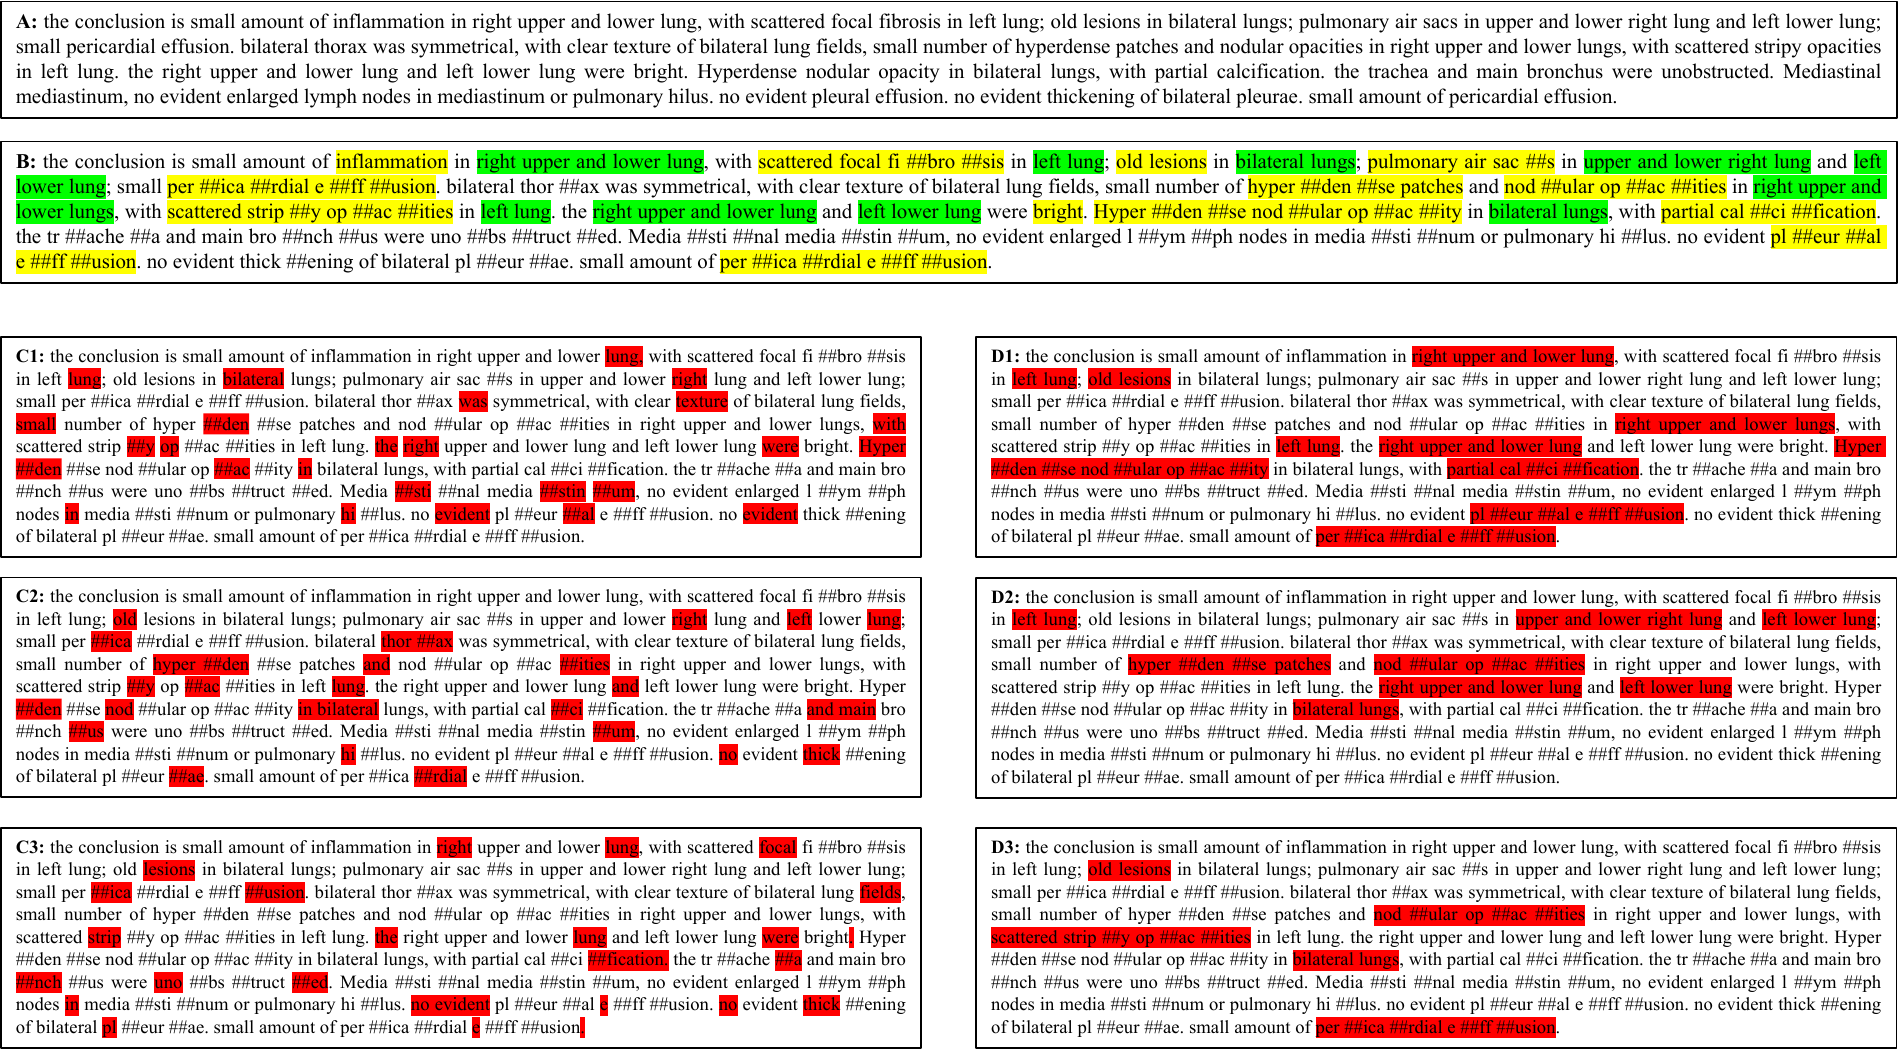}
    \caption{Comparision of random masking and our proposed entity-focused masking.}
    \label{fig:masking}
\end{figure*}

\section{Comparation between Entity-focused masking (EFM) and random masking}
Figure~\ref{fig:masking} illustrates random masking and the proposed entity-focused masking. A denotes the original report, while B denotes the tokenized report using the BERT tokenizer~\cite{devlin2018bert}. The “\#\#” symbol signifies that the subsequent word is a sub-word of the previous one. The entities in B are highlighted in yellow, while the green highlights indicate the distributional information of these entities. C1, C2, and C3 correspond to three randomly masked reports, whereas D1, D2, and D3 represent three reports generated using the entity-focused masking technique (randomly masking either the entity itself or its distributional information). We can see that the words masked through random masking (e.g., "lung", "thick") can be easily inferred based on the context of the report. In contrast, the proposed entity-focused masking approach randomly masks the entity or its distributional information, allowing the network to prioritize more crucial information without compromising contextual coherence. Importantly, our final masking strategy combines entity-focused masking with random masking.








\section{Visualization of language-guided report retrieval}
Figure~\ref{fig:retrival} illustrates an exemplar of language-guided retrieval. In this case, a CT image-report pair is provided, along with nine retrieved X-ray image-report pairs. The values displayed in the top left corner of each X-ray image represent the similarity score between its corresponding report and the given CT report. Notably, the highest similarity score of 0.963 indicates the retrieval of the most semantically relevant report. This highlights the effectiveness of the proposed language-guided retrieval approach in identifying X-ray images that exhibit the closest semantic resemblance to the CT image. Consequently, this approach establishes a solid foundation for facilitating knowledge transfer.

\begin{figure*}
    \centering
    \includegraphics[width=1.0\linewidth]{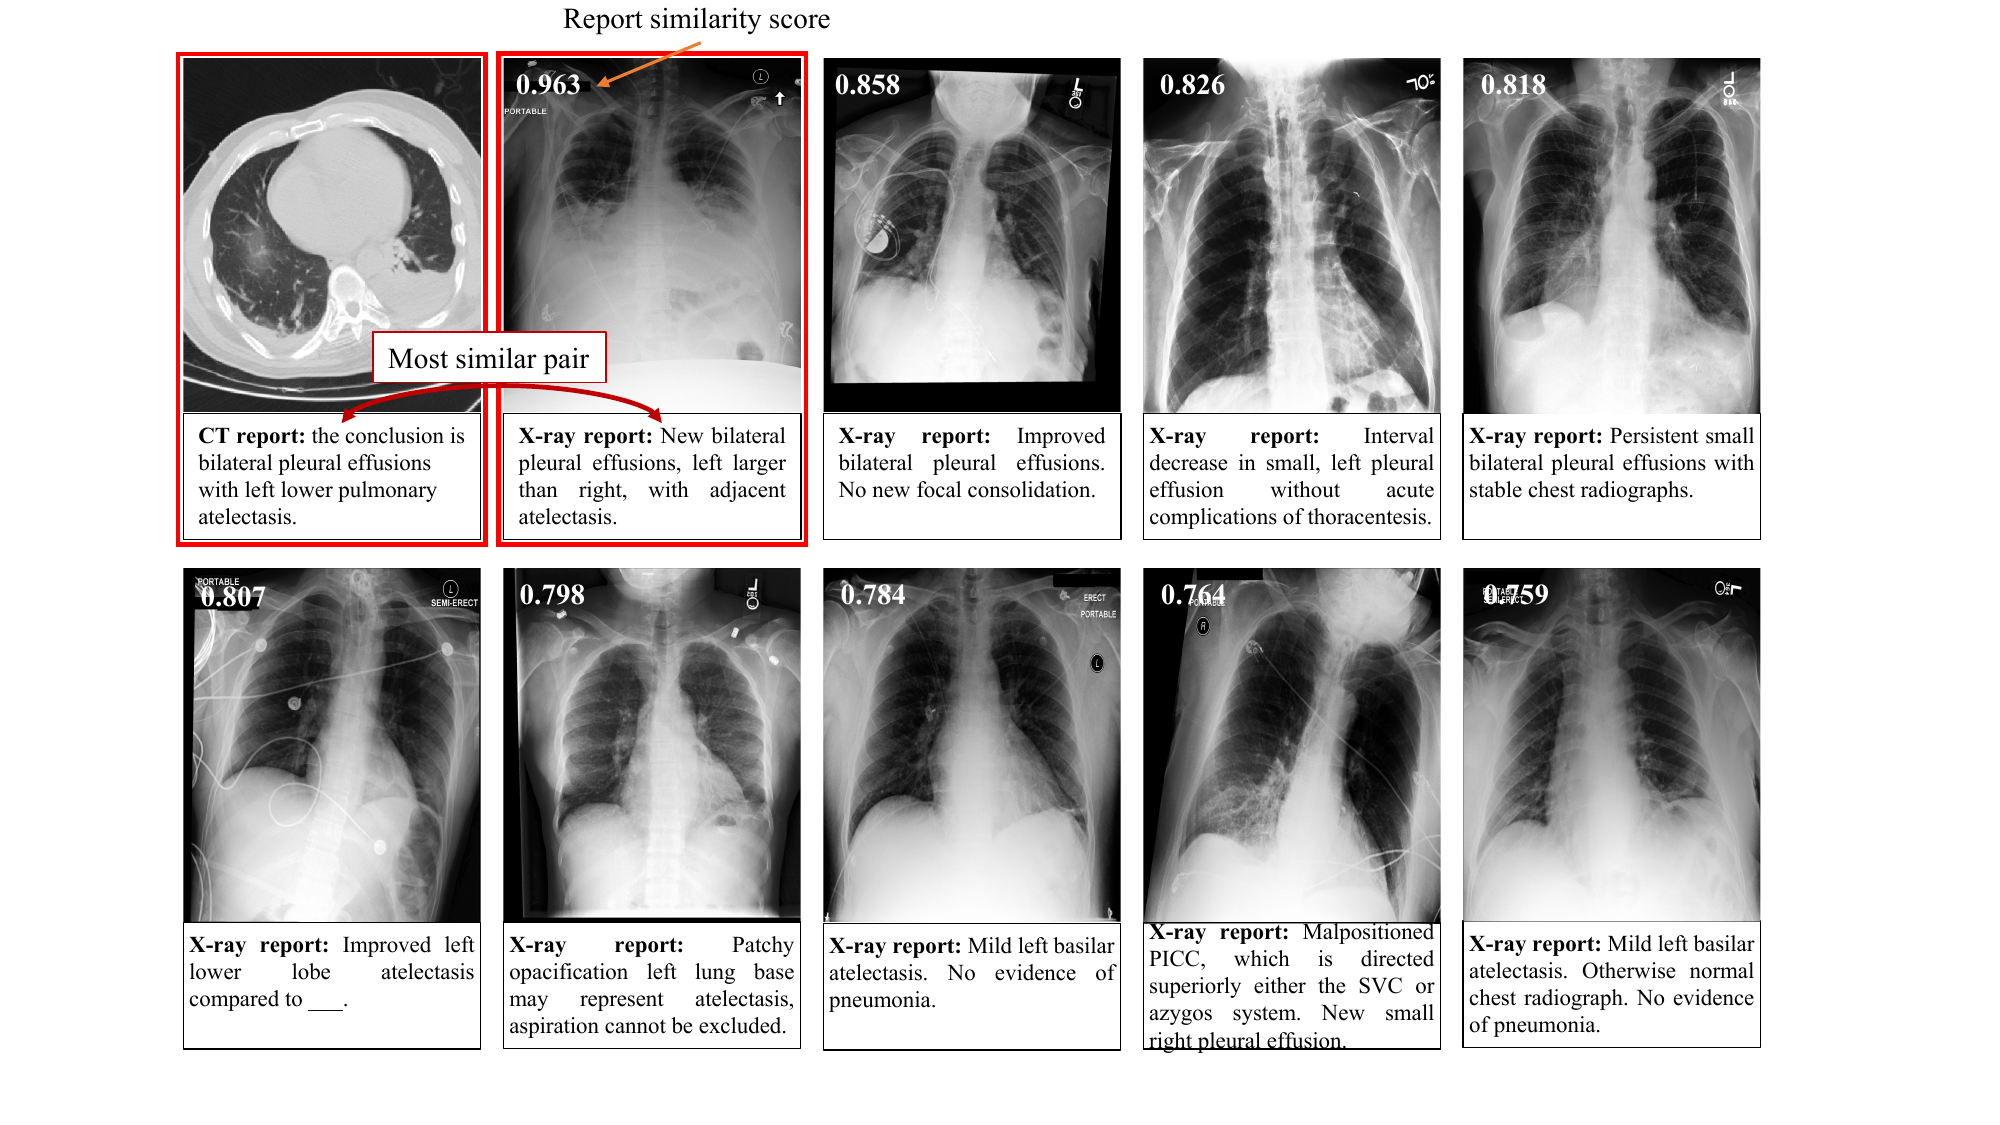}
    \caption{An example of language-guided report retrival. The value in the upper left corner of the X-ray image indicates similarity.}
    \label{fig:retrival}
\end{figure*}
